# Supplementary material for: ProgPrompt: Generating Situated Robot Task Plans using Large Language Models
Source: arXiv:2209.11302 source file (2022-09-22)
Supplement: Supplementary file 1 [file supp.tex]

\begin{figure}[ht]
    \centering
    \vspace{1.5mm}
    \includegraphics[width = \linewidth]{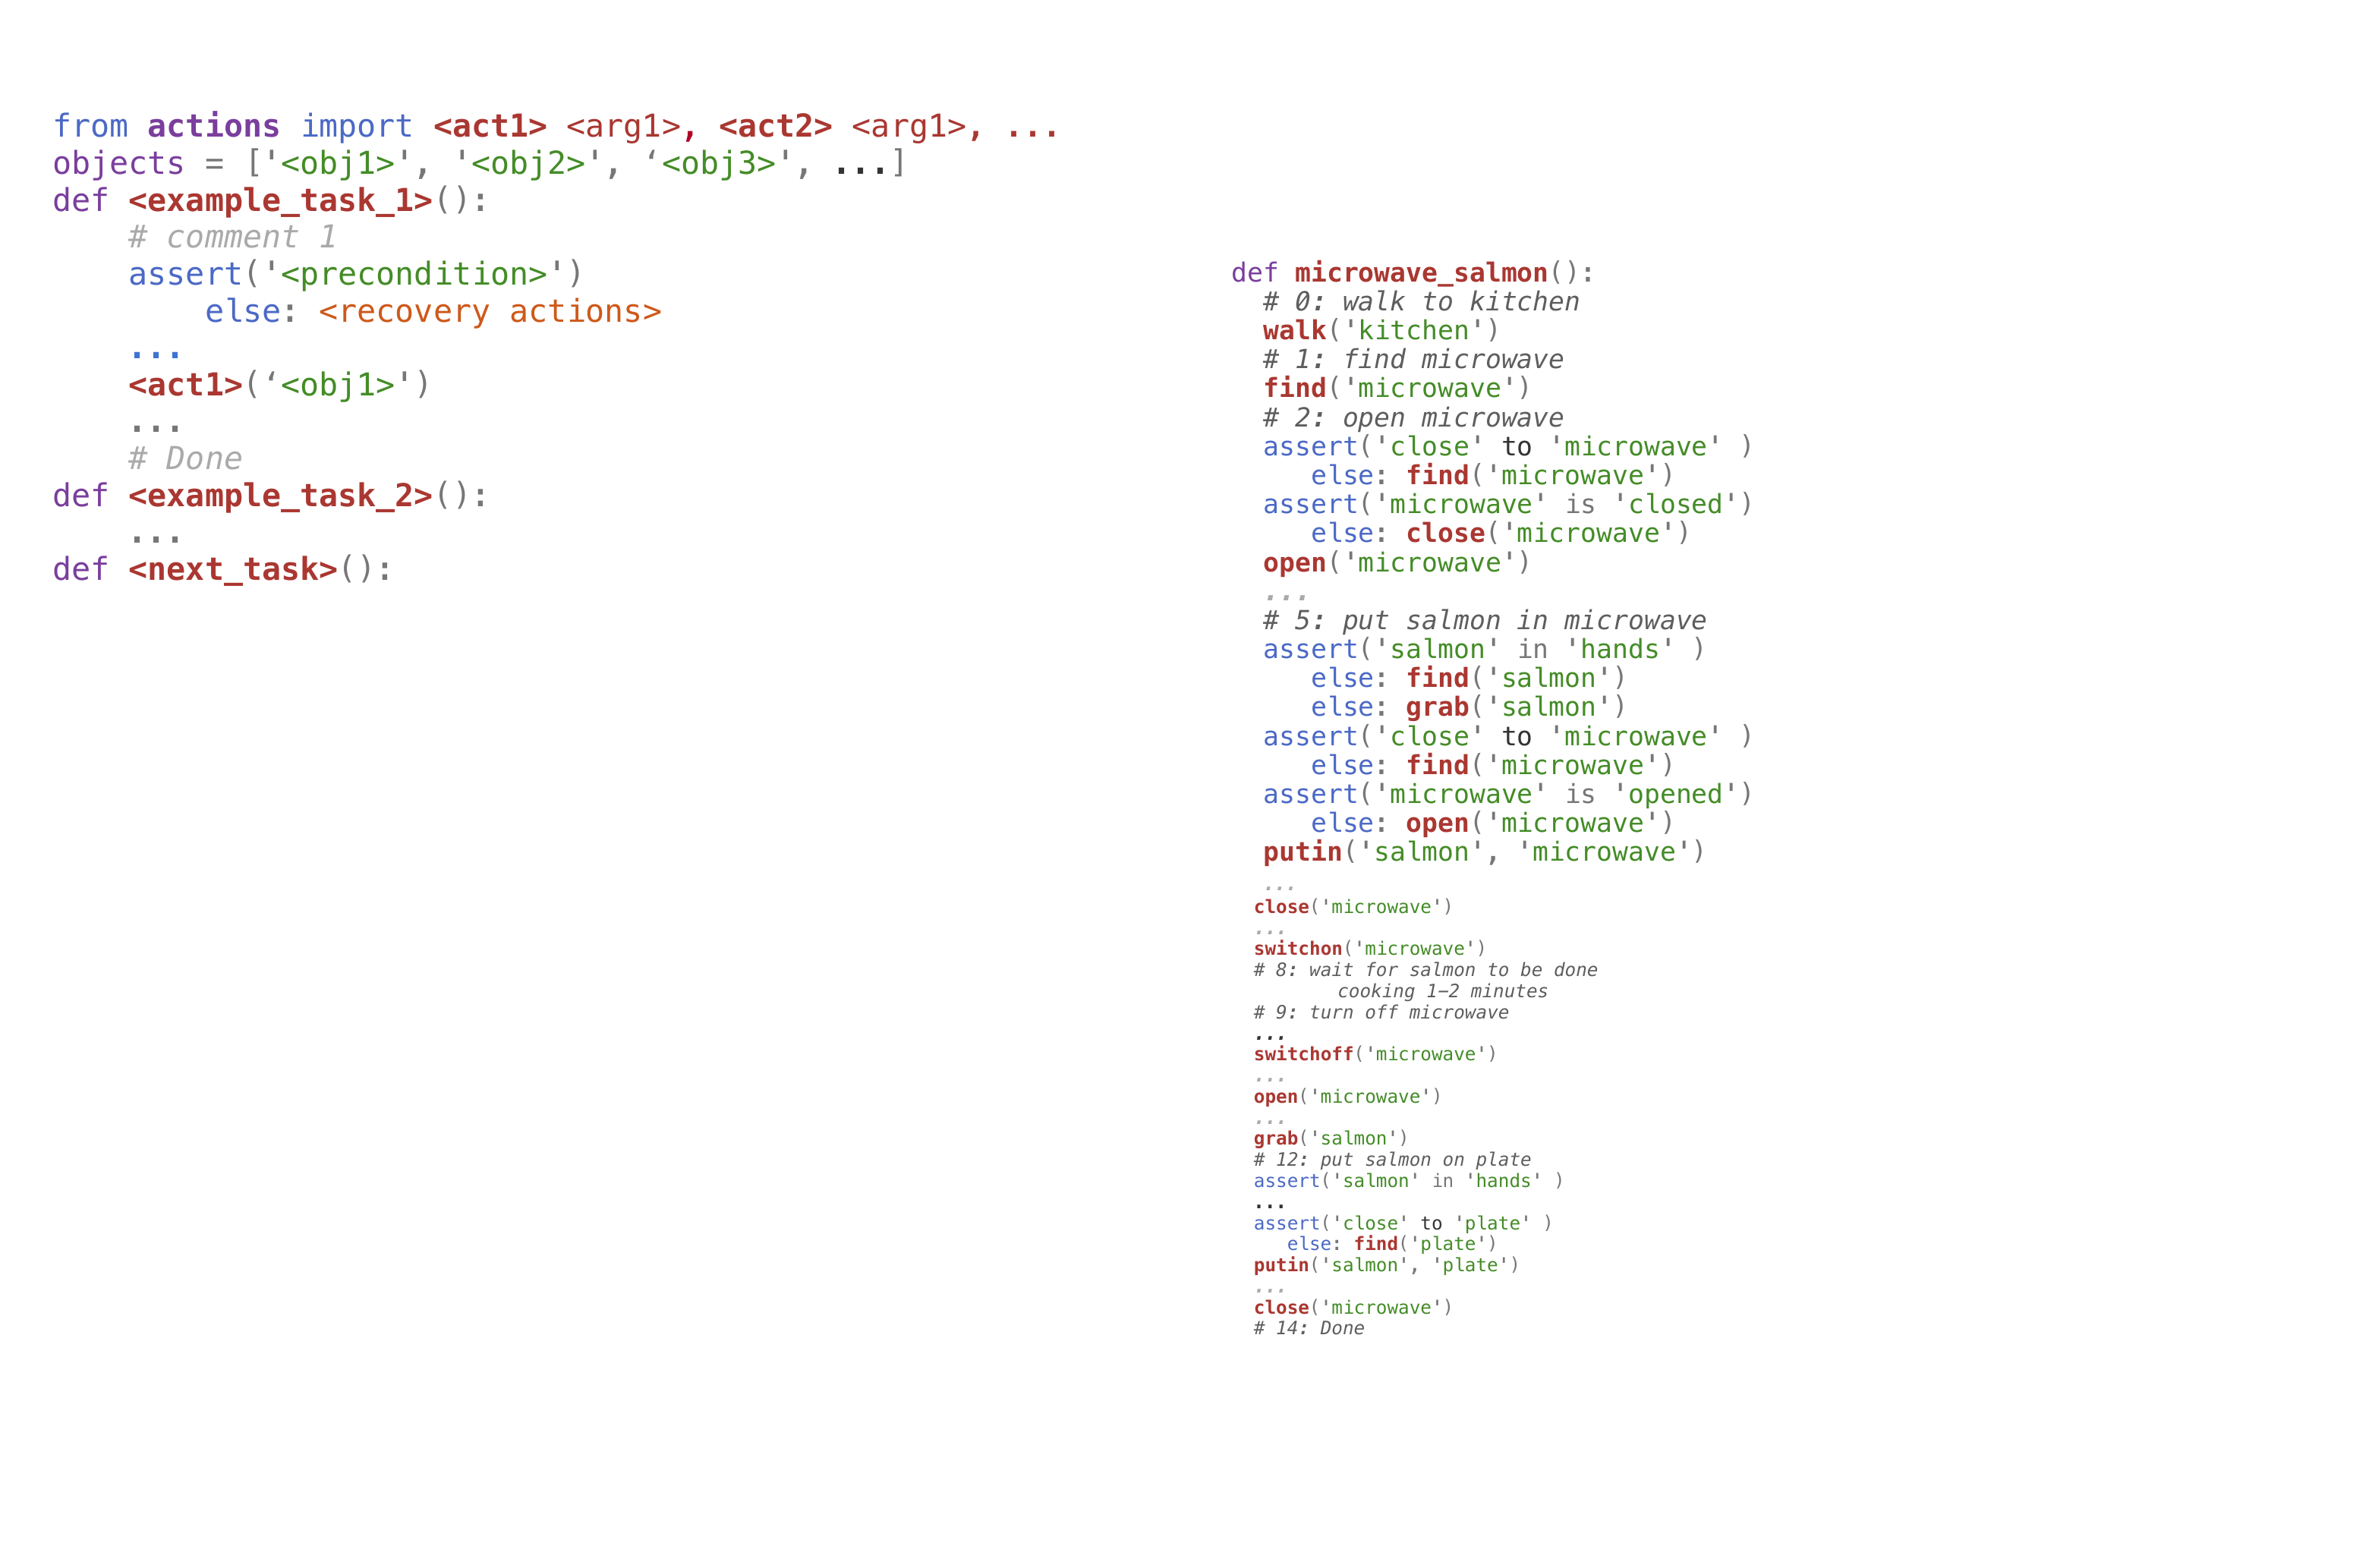}
    \caption{\modelName imports actions, defines an object list, and provides $n$ example tasks.}
    \label{fig:prompt}
\end{figure}

\subsubsection{\textbf{Number of Prompt Examples}} 
We explored different numbers of program examples to include in \modelName prompts (Tab.~\ref{tab:vh_n_examples} using a \textsc{GPT3} backbone with \textsc{Comments} and \textsc{Feedback} included.
We found that including 2 or more example programs led to similar performance, with 3 prompts seeming to hit a local maxima balancing example output (programs) with simulator information, which is given at the beginning of $f_{prompt}$ and so ``lost'' to the model if too much additional text is piled on.

Both fixed and random examples come from the train set of 35 tasks (mentioned in "tasks"). The fixed examples are \texttt{put$\_$wineglass$\_$in$\_$the$\_$kitchen$\_$cabinet}(), \texttt{throw$\_$away$\_$lime}(), \texttt{wash$\_$mug}().  (these are sort of similar to the task in the "test" set), but in case of random example selection from the 35 tasks, there's more variation. \ishika{(should we provide all the tasks here - i created a small set based on what objects/actions were there)}
We also include results for randomized task example selection.  For the evaluation, we removed the examples exactly the same as our test set, while finding a similar plan for the prompt. 
We also get similar results when randomly choosing those 3 example tasks as compared to fixing the example tasks.

\begin{table}[ht]
\caption{Ablation results for task examples in the prompt: Number of prompt examples (\textbf{\#Ex}), using a fixed examples set (\textbf{F}) or chosen randomly (\textbf{R}) per run, for the method \textsc{ProgPrompt-GPT3-Feedback} on \textbf{test} set in \textsc{Env-0}. \#Ex $>1$ improves the performance considerably, while adding more examples or the choice of examples have little effect, indicating the impressive generalization capability of LLMs. We present \#Ex $=3$ as our main result as it achieves the highest \gcr.
}
\label{tab:vh_n_examples}
\begin{center}
\begin{tabular}{llcccc}
    \rowcolor[HTML]{CBCEFB}
    \textbf{\#Ex} & \textbf{F/R} & \sr & \exec & \gcr \\
    \toprule
    1 & F & 0.14$\pm$0.05 & 0.77$\pm$0.02 & 0.47$\pm$0.06 \\
    \rowcolor[HTML]{EFEFEF}
    2 & F & 0.26$\pm$0.10 & 0.80$\pm$0.04 & 0.60$\pm$0.05 \\
    3 & F & $\pmb{0.34}\pm$0.08 & 0.84$\pm$0.01 & $\pmb{0.65}\pm$0.05 \\
    \rowcolor[HTML]{EFEFEF}
    3 & R & 0.28$\pm$0.04 & 0.75$\pm$0.03 & 0.60$\pm$0.03 \\
    5 & F & 0.28$\pm$0.07 & 0.81$\pm$0.04 & 0.58$\pm$0.07 \\
    \rowcolor[HTML]{EFEFEF}
    7 & F & 0.28$\pm$0.07 & $\pmb{0.87}\pm$0.03 & 0.63$\pm$0.05 \\
    \bottomrule
\end{tabular}
\end{center}
\end{table}
